# Supplementary material for: An information theory-based approach for optimal model reduction of biomolecules
Source: arXiv:2004.03988 ancillary file (2020-06-29)
Supplement: Supplementary file 1 [file supp.pdf]

# Supplemental Material for "An information theory–based approach for optimal model reduction of biomolecules"

Marco Giulini,[1,2] Roberto Menichetti,[1,2] M. Scott Shell,[3] and Raffaello Potestio[1,2,*]

[1] *Physics Department, University of Trento, via Sommarive, 14 I-38123 Trento, Italy*
[2] *INFN-TIFPA, Trento Institute for Fundamental Physics and Applications, I-38123 Trento, Italy*
[3] *Department of Chemical Engineering, University of California Santa Barbara, Santa Barbara, California 93106, USA*

(Dated: June 29, 2020)

This Supplemental Material contains:

1. a quantitative analysis of the all-atom MD simulations of the three proteins investigated in this work
2. additional figures about the CG representations that minimise the mapping entropy
3. an analysis of the relation between the size and mobility of residues and the conservation probability of their atoms
4. an assessment of the results' stability with respect to the duration of the MD trajectory.

### Parameters and analysis of the all-atom MD simulations

MD simulations in this work are performed using Gromacs 2018 package [1, 2] and the Amber99sb-ildn force field [3], with a timestep $\delta t = 2$ fs. We apply the LINCS algorithm to constrain all the bonds involving hydrogen atoms [4], and treat long-range electrostatics by means of the *Particle Mesh Ewald* method [5].

We first equilibrate each protein structure at 300 K in the canonical ($NVT$) ensemble by means of a stochastic velocity rescaling thermostat [6], relying on a coupling constant $\tau_T = 0.1$ ps. Subsequently, a further equilibration simulation sets the pressure of each system at $P = 1$ bar, achieved by superimposing to the thermostat a Parrinello-Rahman barostat ($\tau_P = 2$ ps) [7]. We then extract from the $NPT$ equilibration run of each protein a configuration whose volume $V$ is compatible to the average volume $\langle V \rangle$, the latter being calculated from the corresponding $NPT$ run. Such configurations are employed as initial conditions for production simulations of 200 ns in $NVT$.

Fig. S1 describes the simulations in terms of RMSD and Root Mean Square Fluctuation (RMSD). Both quantities are computed with respect to a reference conformation, that we choose to be the first frame of the trajectory.

We observe that TAM shows rather abrupt transitions in both graphs: from the point of view of RMSD this suggests the presence of local conformational rearrangements that occur over the time scales of few nanoseconds, while such a behavior for RMSF implies that there are huge differences between atoms that are contiguous in the protein sequence.

As for AKE, we select two reference conformation for the RMSD calculation: in addition to the first frame, we compute it also with respect to its closed structure (1AKE): it is possible to notice that peaks in one time series correspond to local minima in the other, thus suggesting the presence of *intermediate* configurations between the two. Therefore AKE explores some conformations that share some similarity with the structure of 1AKE, although a full conformational transition is never observed. This *flavour* of the closed conformation may explain our algorithm's capability of identifying residues important for stabilizing 1AKE.

Finally, the RMSD of AAT with respect to its first frame seems to increase steadily, while staying well below the value of 0.3 nm for all the 200 ns of trajectory. This behavior, combined with the low values of RMSF shown below, is index of a very compact structure that is still far from reaching equilibrium. The region with the peak in local fluctuations is the one involved in the conformational rearrangement of AAT: these atoms spend the entire duration of the MD simulation wiggling in the solvent, probably carrying very few information content from the point of view of energetics. This can be the main reason behind the fact that this region is heavily coarse-grained by the optimisation procedure.

### Additional figures on optimised mappings

Here we report some additional data about the solutions we obtain from our optimisation procedure. In particular, Fig. S2 shows, for all investigated proteins, a set of 100 transitions (see Fig. 2 in the main text) between the three couples of optimal mappings identified throughout the optimisation algorithm presenting the lowest values of $\Sigma$. Fig. S3 displays, in analogy with Fig. 4 in the main text, the distribution of conservation probabilities for Adenylate Kinase and $\alpha - 1$ antitrypsin.

We also investigated possible correlations between an atom's conservation probability $P_{cons}$ and its mobility, which is well described by the RMSF extracted from the MD trajectory (Fig. S1). From Fig. S4 we can observe a weak degree of correlation: in particular, atoms with a high value of $P_{cons}$ usually have a large mobility as well. On the contrary, though, not all atoms with large RMSF

* raffaello.potestio@unitn.it

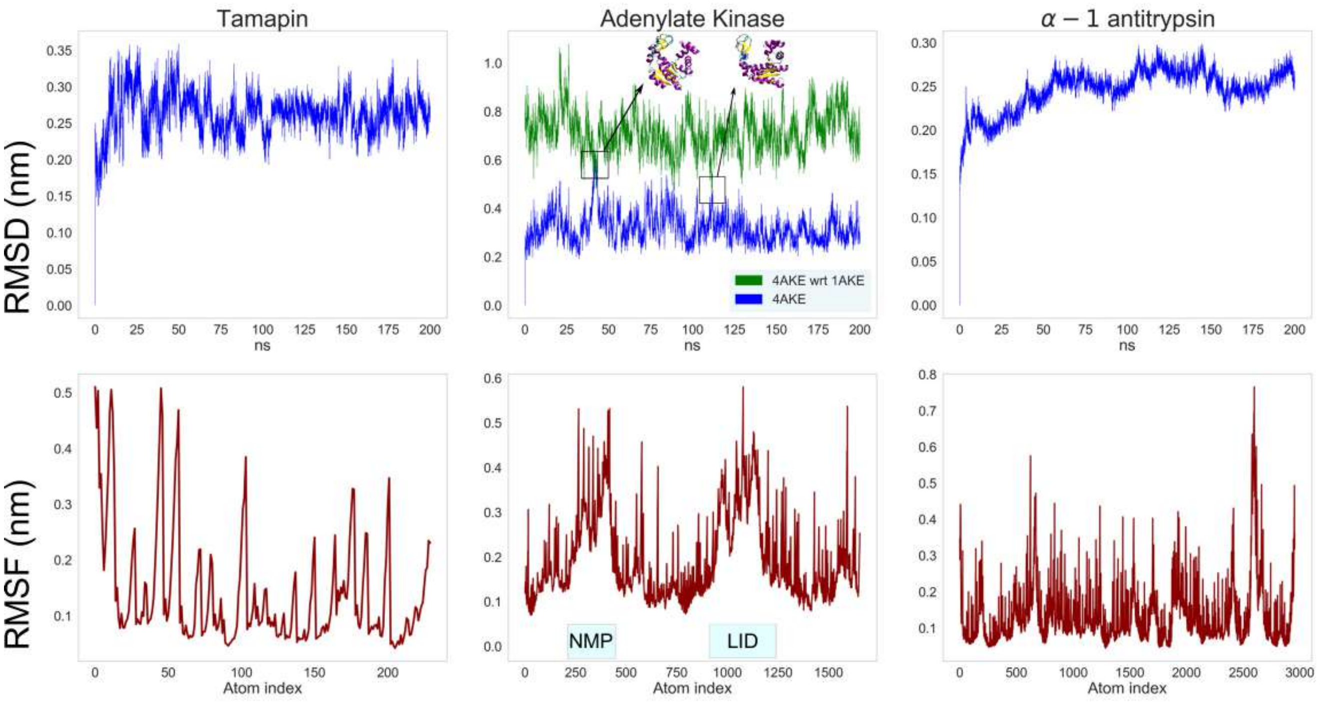


FIG. S1: RMSD (top) and RMSF (bottom) for the three protein of interest. RMSD values are always calculated with respect to the first frame of the trajectory. For adenylate kinase we display also the RMSD with respect to the PDB of the closed conformation (4AKE wrt 1AKE, monomeric structure). LID and NMP domains are also highlighted in the RMSF plot.

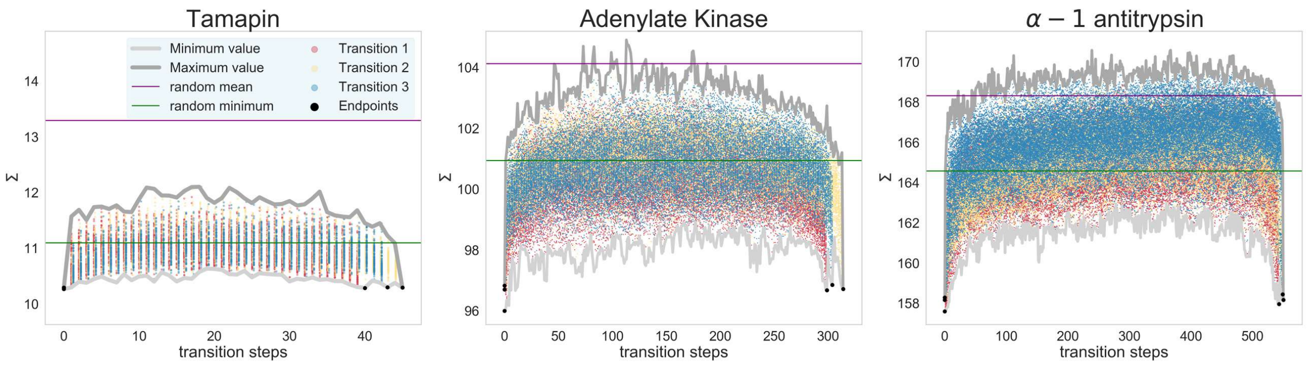


FIG. S2: Values of the mapping entropy $\Sigma$ $[kJ/\mathrm{mol}/K]$ of mappings connecting optimal solutions. In each plot, one per protein under examination, 100 transitions have been sampled between the three next-to-lowest-$\Sigma$ pairs of optimal mappings at $N = N_{\alpha\beta}$. Black dots indicate initial and final endpoints for paths constructed by swapping pairs of atoms between them (coloured dots). In each plot, horizontal lines represent the mean (violet) and minimum (green) $S_{map}$ obtained from the corresponding distribution of random mappings presented in Fig. 1 of the main text. The behaviour illustrated in Fig. 2 of the main text is preserved.

are conserved with high probability, since highly mobile atoms can either be involved in several interactions, or be exposed on the protein's surface and wiggle in the solvent without having contacts with other residues.

From the inspection of Fig. S4 we can underline the notable case of residue ARG13 of TAM. While the terminal nitrogen NH2 is almost always included in the optimised mapping ($P_{cons} = 0.96$), NH1 possesses a negligible conservation probability ($P_{cons} = 0.04$). Interestingly, in one of the two optimised solutions in which NH2-ARG13

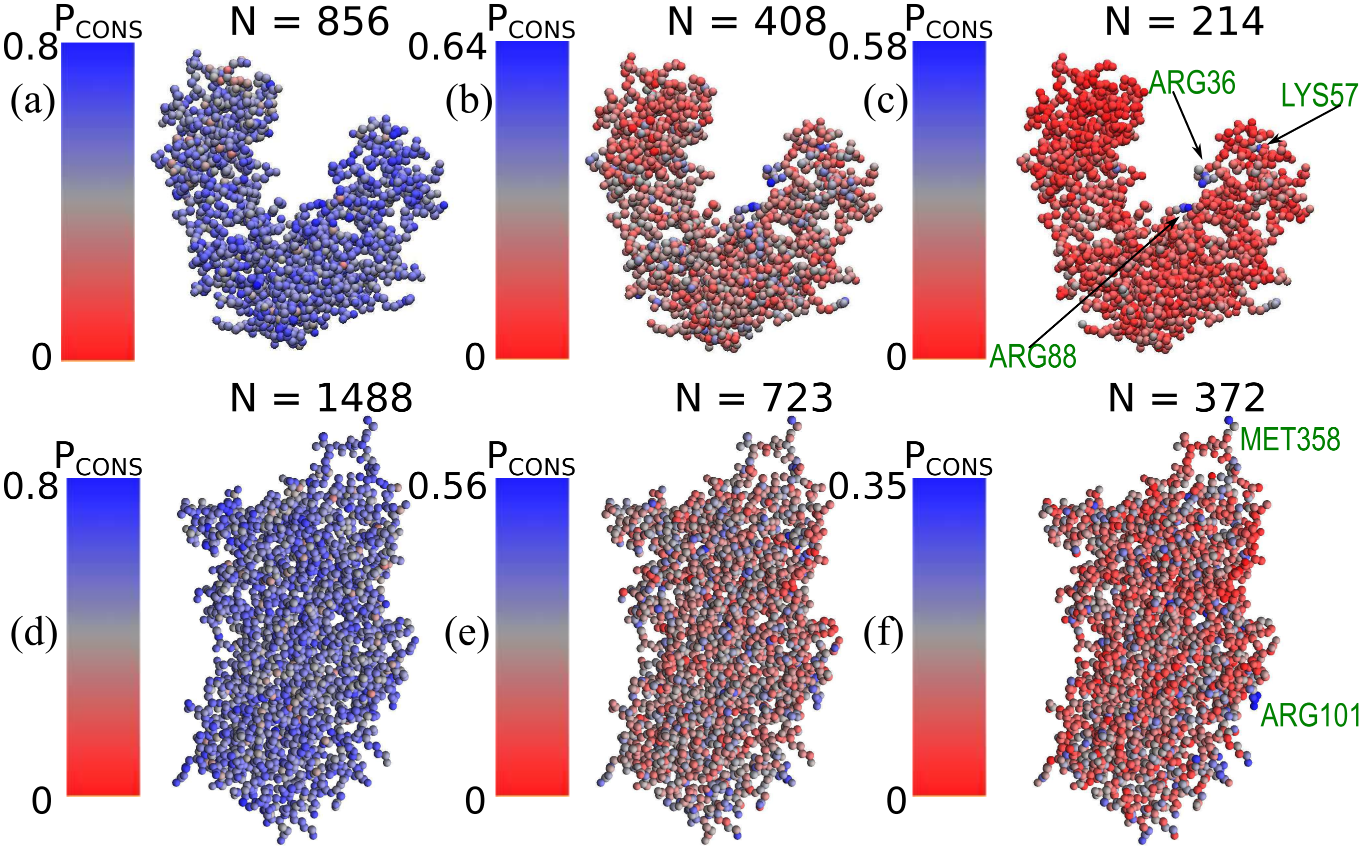


FIG. S3: Adenylate Kinase [(a),(b) and (c)], and $\alpha - 1$ antitrypsin [(d), (e) and (f)]: probability of conserving sites over the optimised solutions as a function of the number $N$ of retained sites. The residues containing those atoms that are conserved with the highest probability have been explicitly indicated in fiugre.

is absent, we observe the presence of NH1-ARG13, thus suggesting that one of the two nitrogens always has to be retained, NH2 being the preferred one.

In Fig. S5 we report average values and standard deviations of $P_{cons}$ for each atom of selected amino acids in our proteins of interest. We consider the 3, 13 and 7 arginine residues of TAM, AKE and AAT, respectively. We expand this analysis including glutamic acid monomers for TAM (3 residues), lysine amino acids for AKE (18 residues) and MET amino acids for AAT (10 residues). In all the inspected cases the algorithm is more likely to conserve terminal atoms than elements of backbone or of the first part of the side chain, such as the beta carbon (CB). More importantly, the standard deviation of $P_{cons}$ increases consistently with the distance from the backbone chain. A possible explanation for this phenomenon could lie in the fact that terminal atoms of amino acids with long side chains can be considered either extremely relevant or completely negligible for the mapping. In particular, when the residue takes part to highly energetic structural fluctuations, like ARG88 in AKE, at least one of its terminal atoms, which are usually the main actors of such interactions, is very likely conserved.

As for the non-terminal elements of the monomer, we observe lower standard deviations: one or two of them might be retained, but the specific choice is less crucial from the point of view of the mapping, since they are less likely to be directly involved in residue-residue interactions.

## Application of the protocol to the last 100 ns of MD trajectories

Here we briefly summarise the results of the measurement and minimisations of mapping entropy in all three proteins under examination, taking as sampled structures the configurations extracted from the last 100 ns of MD trajectories. Frames are separated by 10 ps in order to consider $10^4$ configurations, as we do in the work presented in the main text. $5 \times 10^3$ of them are already included in the 200 ns sampling, while the other half of them consists of new snapshots. The data that follow represent a first assessment of how the results of the protocol illustrated in this paper depend on the extent of the sampling.

Fig. S6, S7 and S8 show the results of the calculations performed as in the main text, applied to the set

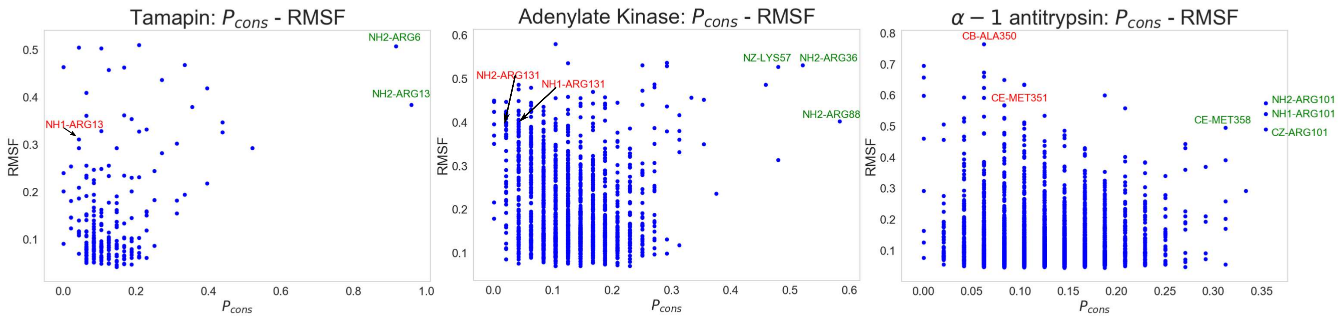


FIG. S4: Atom-wise comparison between RMSF and $P_{cons}$ (calculated at $N = N_\alpha$) for the three proteins of interest. We highlighted in green the most conserved atoms, for which the RMSF is always non negligible. We also pinpoint in red highly mobile atoms that are almost never included in the optimised solution.

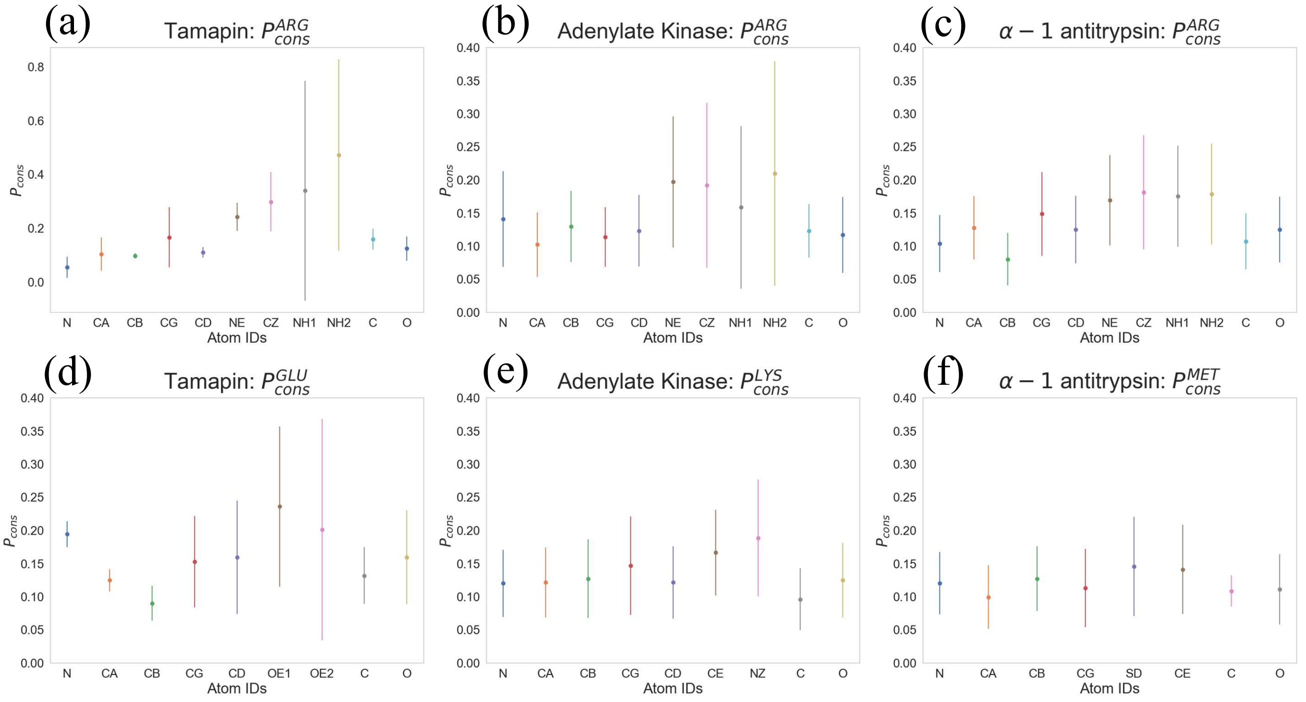


FIG. S5: Plot of average $P_{cons}$ with its standard deviation for each atom of arginine residues for the three considered proteins [(a),(b) and (c)]. We add GLU atoms [(d)] for TAM, LYS atoms [(e)] for AKE and MET atoms [(f)] for AAT. Values on the y-axis ($P_{cons}$) change between the plots. With the exception of figure (a), values on y-axis always range from 0.0 to 0.4.

of shorter trajectories. We restrict ourselves to the case $N = N_\alpha$. From Fig. S7 we can observe that the range of $\Sigma$ values covered by the optimised and random mappings is shifted towards lower ones with respect to those reported in Fig. 1 of the main text. Consistently with the latter, the $C_\alpha$ mapping is on the far right region of the distribution of random mappings, as it was the case employing 200 ns of sampling.

Regarding the subset of atoms that are more conserved by the optimisation procedure, we deem it useful to highlight the changes protein by protein:

- **[TAM]**: the terminal atoms in the arginine residues ARG6 and ARG13 are conserved with medium-to-high values of $\Sigma$ ($P_{\rm cons}({\rm CZ, ARG13}) = 0.58$, $P_{\rm cons}({\rm NH2, ARG6}) = 0.46$, $P_{\rm cons}({\rm CZ, ARG6}) = 0.42$). These values are lower than the ones observed with 200 ns of conformational sampling. Interestingly, the atoms retained with higher probabilities in the terminal regions of these arginine residues are not the ones identified in the main text. Overall, the atoms with highest $P_{\rm cons}$ are the terminal oxygens of GLU24 ($P_{\rm cons}({\rm OE1, GLU24}) = 0.71$, $P_{\rm cons}({\rm OE2, GLU24}) = 0.69$);
- **[AKE]**: from Fig. S6 we can see that, as in

the case reported in the main text, the external portion of the LID domain is heavily coarse-grained. Looking at specific atoms, ARG88 is retained with values of $P_{\text{cons}}$ ($P_{\text{cons}}(\text{NH2}, \text{ARG88}) = 0.79$, $P_{\text{cons}}(\text{CZ}, \text{ARG88}) = 0.65$) even higher than those obtained with 200 ns of sampling. Instead, ARG36 and LYS57 are well conserved but without the peaks in probability that we observed in the main text. This result may suggest that, in the full simulation, ARG88 is always involved in highly energetic medium-to-large scale rearrangements, while the other two residues play a less prominent role in the last 100 ns;

- **[AAT]**: while the residue ARG101 does not possess atoms with $P_{\text{cons}}$ higher than 0.21, MET358 terminal atoms are well conserved throughout the optimised solutions ($P_{\text{cons}}(\text{SG}, \text{MET358}) = 0.25$ , $P_{\text{cons}}(\text{CE}, \text{MET358}) = 0.25$). In the case of AAT 100 ns of MD sampling seem to be too few to extract relevant information from the trajectory.

The evaluation of the dependence of mapping entropy values on the duration and other features of the employed MD trajectories is a fundamental step to critically assess advantages and limitations of the method. It is reasonable to expect that, as it is the case with any approach that relies on MD simulations as input data, a variation of the latter induces a variation of the results. This variation can be made use of to investigate the features of the input, e.g. in the present case different mappings can emerge from trajectories sampling different structural basins.

Although this is only a preliminary analysis, the results described above suggest that several features of the optimised mappings are retained even when we employ a different set of configurations. The usage of the last 100 ns of the trajectories has shown small variations, coherent with the different duration of the input and the stochastic nature of the optimisation procedure, as well as an overall consistent pattern of results, which demonstrates the solidity of the approach.


[1] D. Van Der Spoel, E. Lindahl, B. Hess, G. Groenhof, A. E. Mark, and H. J. Berendsen, "Gromacs: fast, flexible, and free," *Journal of computational chemistry*, vol. 26, no. 16, pp. 1701–1718, 2005.

[2] M. J. Abraham, T. Murtola, R. Schulz, S. Páll, J. C. Smith, B. Hess, and E. Lindahl, "Gromacs: High performance molecular simulations through multi-level parallelism from laptops to supercomputers," *SoftwareX*, vol. 1, pp. 19–25, 2015.

[3] K. Lindorff-Larsen, S. Piana, K. Palmo, P. Maragakis, J. L. Klepeis, R. O. Dror, and D. E. Shaw, "Improved side-chain torsion potentials for the amber ff99sb protein force field," *Proteins: Structure, Function, and Bioinformatics*, vol. 78, no. 8, pp. 1950–1958, 2010.

[4] B. Hess, H. Bekker, H. J. Berendsen, and J. G. Fraaije, "Lincs: a linear constraint solver for molecular simulations," *Journal of computational chemistry*, vol. 18, no. 12, pp. 1463–1472, 1997.

[5] U. Essmann, L. Perera, M. L. Berkowitz, T. Darden, H. Lee, and L. G. Pedersen, "A smooth particle mesh ewald method," *The Journal of chemical physics*, vol. 103, no. 19, pp. 8577–8593, 1995.

[6] G. Bussi, D. Donadio, and M. Parrinello, "Canonical sampling through velocity rescaling," *The Journal of chemical physics*, vol. 126, no. 1, p. 014101, 2007.

[7] M. Parrinello and A. Rahman, "Polymorphic transitions in single crystals: A new molecular dynamics method," *Journal of Applied physics*, vol. 52, no. 12, pp. 7182–7190, 1981.

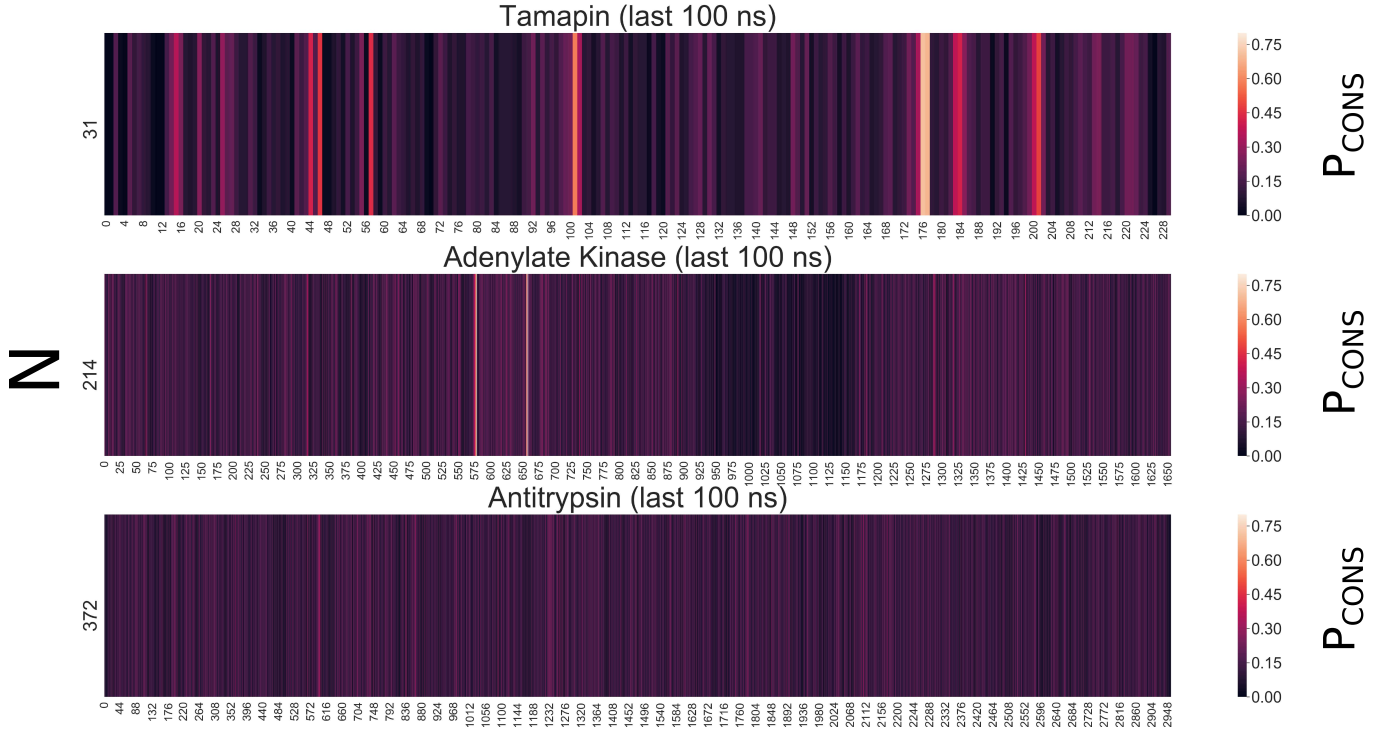


FIG. S6: Probability $P_{\text{cons}}$ that a given atom is retained in the optimal mapping for each analysed protein, expressed as a function of the atom index. Atoms are ordered according to their number in the PDB file. These probabilities are obtained using, for each of the three proteins under examination, a number of retained sites equal to the number of $C_\alpha$ atoms, and performing thermal averages on the second half (100 ns) of the MD trajectory employed in this study.

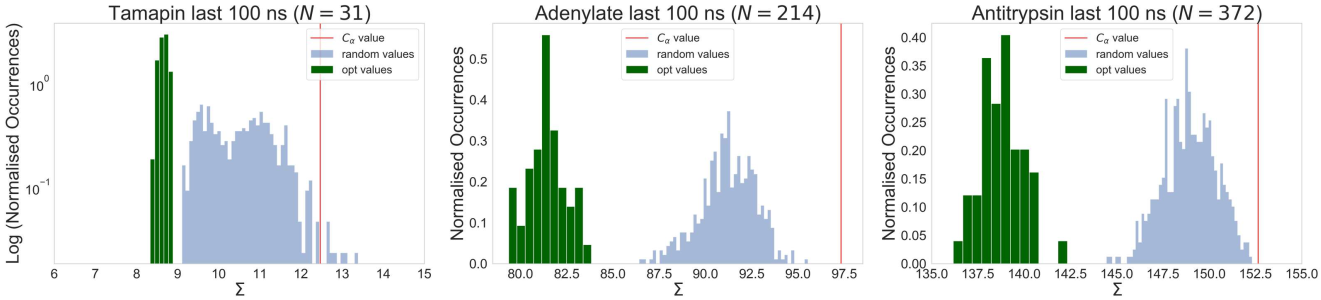


FIG. S7: Distributions of the values of mapping entropy $\Sigma$ $[kJ/\text{mol}/K]$ for random mappings (light blue histograms) and optimised solutions (green histograms) for each analysed protein. These data are obtained using, for each of the three proteins under examination, a number of retained sites equal to the number of $C_\alpha$ atoms, and performing thermal averages on the second half (100 ns) of the MD trajectory employed in this study.

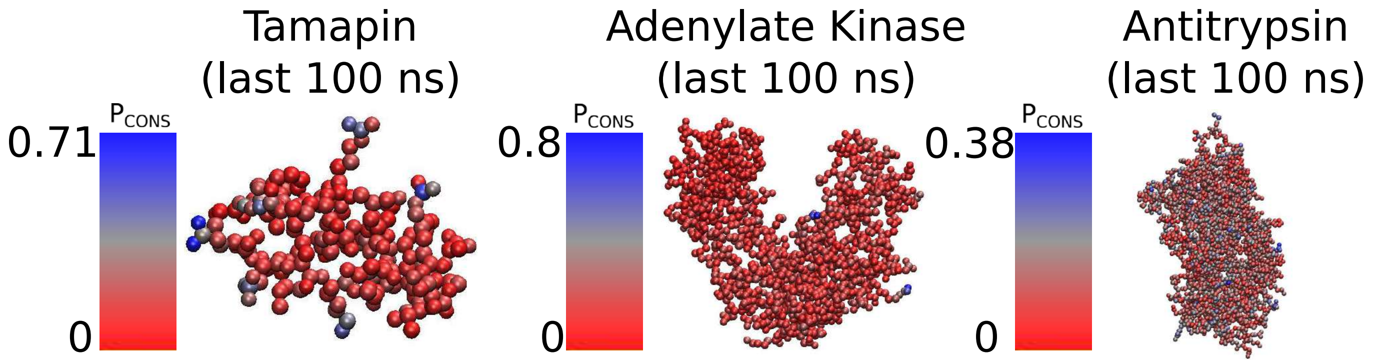


FIG. S8: $P_{\text{cons}}$ of conserving atoms calculated taking into account only the last 100 ns of the MD simulations. A visual comparison with Fig. 4 in the main text (for TAM) and Fig. S3 (for AKE and AAT) can show the differences between the two cases.
